# Supplementary material for: Robust No-Regret Learning in Min-Max Stackelberg Games
Source: arXiv:2203.14126 source file (2022-04-13)
Supplement: Supplementary file 1 [file algos.tex]

\section{Pseudo-Code for Algorithms}\label{sec-app:algos}

\begin{algorithm}[H]
\caption{Max-Oracle Gradient Descent}
\label{alg:mogd}
\textbf{Inputs:} $\outerset, \innerset, \obj, \constr, \learnrate, \outeriters, \outer^{(0)}$ \\ 
\textbf{Output:} $\outer^{*}, \inner^{*}$
\begin{algorithmic}[1]
\For{$\outeriter = 1, \hdots, \outeriters$}
    \State Find $\inner^*(\outer[][\iter -1]) \in \br[\innerset](\outer[][\iter -1])$ 
    \State Set $\inner^{(\outeriter-1)} = \inner^*(\outer[][\iter -1])$ 
    \State Set $\langmult^{(\outeriter-1)} = \langmult^*(\outer^{(\outeriter-1)}, \inner^{(\outeriter-1)})$
    \State Set $\outer^{(\outeriter)} = \project[\outerset] \left[ \outer^{(\outeriter-1)} - \learnrate[\outeriter] \grad[\outer] \lang[{\outer^{(\outeriter-1)}}]\left( \inner^{(\outeriter-1)}, \langmult^{(\outeriter-1)}\right) \right]$
\EndFor
\State Set $\avgouter[][\numiters] = \frac{1}{\numiters} \sum_{\iter = 1}^\numiters \outer[][\iter]$
\State Set $\inner^*(\avgouter[][\numiters]) \in \br[\innerset](\avgouter[][\numiters])$
\State \Return $(\avgouter[][\numiters], \inner^*(\avgouter[][\numiters]))$
\end{algorithmic}
\end{algorithm}

\begin{algorithm}[H]
\caption{Lagrangian Gradient Descent Ascent (LGDA)}
\label{alg:lgda}
\textbf{Inputs:} $\langmult^*, \outerset, \innerset, \obj, \constr,  \learnrate[][\outer], \learnrate[][\inner], \numiters,  \outer^{(0)}, \inner^{(0)}$ \\ 
\textbf{Output:} $\outer^{*}, \inner^{*}$
\begin{algorithmic}[1]
\For{$\iter = 1, \hdots, \numiters -1$}    
    \State Set $\outer^{(\iter +1)} = \project[\outerset] \left( \outer^{(\iter)} - \learnrate[\iter][\outer] \grad[\outer] \lang[{\outer[][\iter]}](\inner[][\iter], \langmult^*)
    % \left[\grad[\outer] \obj (\outer^{(\iter)}, \inner^{(\iter)}) + \sum_{\numconstr = 1}^\numconstrs \langmult[\numconstr]^* \grad[\outer]  \constr[\numconstr](\outer^{(\iter)}, \inner^{(\iter)}) \right] 
    \right)$

    \State Set $\inner^{(\iter +1)} = \project[{
    \innerset
    }] \left( \inner^{(\iter)} + \learnrate[\iter][\inner] \grad[\inner] \lang[{\outer[][\iter]}](\inner[][\iter], \langmult^*)
    % \left[ \grad[\inner] \obj (\outer^{(\iter)}, \inner^{(\iter)}) + \sum_{\numconstr = 1}^\numconstrs \langmult[\numconstr]^* \grad[\inner]  \constr[\numconstr](\outer^{(\iter)}, \inner^{(\iter)}) \right] 
    \right)$ 
\EndFor
\State \Return $\{(\outer[][\iter], \inner[][\iter])\}_{\iter= 1}^\numiters$
\end{algorithmic}
\end{algorithm}

\begin{algorithm}[H]
\caption{Dynamic t\^atonnement}
\label{alg:dynamic_max_oracle_gd}
\textbf{Inputs:} $\numiters, \{(\util^{(\iter)}, \budget^{(\iter)}, \supply^{(\iter)}) \}_{\iter =1}^\numiters, \learnrate,  \price^{(0)}, \delta$ \\ 
\textbf{Output:} $\outer^{*}, \inner^{*}$
\begin{algorithmic}[1]
\For{$\iter = 1, \hdots, \numiters -1$}
    % \State Obtain market parameters 
    \State For all $\buyer \in \buyers$, find $\allocation[\buyer]^{(t)} \in \argmax_{\allocation[\buyer] \in \R^\numgoods_+:\allocation[\buyer]\cdot \price^{(\iter-1)} \leq \budget[\buyer]^{(\iter)}} \util[\buyer](\allocation[\buyer])$
    % $ s.t. $\util[\buyer]^{(\iter)} (\allocation[\buyer]^{(\iter)})) \geq \max_{\allocation[\buyer]:\allocation[\buyer]\cdot \price^{(\iter-1)} \leq \budget[\buyer]^{(\iter)}} \util[\buyer]^{(\iter)}(\allocation[\buyer]) - \delta$ and $\allocation[\buyer]^{(\iter-1)} \cdot \price^{(\iter-1)} \leq \budget[\buyer]^{(\iter)}$ 
    \State Set $\price^{(\iter)} =\project[\R_+^\numgoods]\left( \price^{(t-1)} - \learnrate[t](\supply^{(\iter)} - \sum_{\buyer \in \buyers} \allocation[\buyer]^{(t)})
    \right)$
\EndFor
\State \Return $(\price^{(\iter)}, \allocation^{(\iter)})_{\iter = 1}^\numiters$ 
\end{algorithmic}
\end{algorithm}

\begin{algorithm}[H]
\caption{Dynamic Myopic Best-Response Dynamics}
\label{alg:dynamic_lgda}
\textbf{Inputs:} $\{(\util^{(\iter)}, \budget^{(\iter)}, \supply^{(\iter)}) \}_{\iter =1}^\numiters, \learnrate[][\price], \learnrate[][\allocation], \numiters, \allocation^{(0)}, \price^{(0)}$ \\ 
\textbf{Output:} $\outer^{*}, \inner^{*}$
\begin{algorithmic}[1]
\For{$\iter = 1, \hdots, \numiters -1$}
    % \State Obtain market parameters $\util^{(\iter)}, \budget^{(\iter)}, \supply^{(\iter)}$
    \State Set $\price^{(\iter +1)} = \project[\R_+^\numgoods]\left(
    \price^{(t)} - \learnrate[t][\price](\supply^{(\iter)} - \sum_{\buyer \in \buyers} \allocation[\buyer]^{(t)})
    \right)$
    % \sadie{Should this be $\project[\R_+^\numgoods]\left(\price^{(t)} - \learnrate[t][\outer](\supply^{(\iter)} - \sum_{\buyer \in \buyers} \allocation[\buyer]^{(t)})\right)$?}
    \State For all $\buyer \in \buyers$, set $\allocation[\buyer]^{(\iter +1)} = \project[\R^\numgoods_+] \left( \allocation[\buyer]^{(\iter)} + \learnrate[\iter][\allocation]  \left( \frac{\budget[\buyer]^{(\iter)}}{\util[\buyer]^{(\iter)}\left(\allocation[\buyer]^{(\iter)}\right)} \grad[{\allocation[\buyer]}] \util[\buyer]^{(\iter)}\left(\allocation[\buyer]^{(\iter)}\right) - \price^{(\iter)} \right)\right)$
    % \sadie{$\learnrate[][\allocation]?$ }
\EndFor
% \State Draw $(\widehat{\price}, \widehat{\allocation})$ uniformly at random from $\{(\price^{(\iter)}, \allocation^{(\iter)}\}_{\iter = 1}^\iters$
\State \Return $(\price^{(\iter)}, \allocation^{(\iter)})_{\iter = 1}^\numiters$ 
\end{algorithmic}
\end{algorithm}
